# Supplementary material for: A Comparative Study of Machine Learning Models Predicting Energetics of Interacting Defects
Source: arXiv:2403.13243 source file (2024-03-20)
Supplement: Supplementary file 1 [file appendix.tex]

Data
